# Supplementary material for: In-Context Learning on a Budget: A Case Study in Token Classification
Source: arXiv:2406.13274 source file (2025-01-28)
Supplement: Supplementary file 1 [file app_d_additional_results.tex]

In this section we report additional results on NER using a recently introduced dataset, Universal NER (UNER; \citealp{mayhew2023universal}). The input texts are sourced from the UD dataset. We use the same models, prompts and pool sizes as used for Ontonotes.

\begin{figure*}[tb!]
    \centering
    \includegraphics[width=\textwidth]{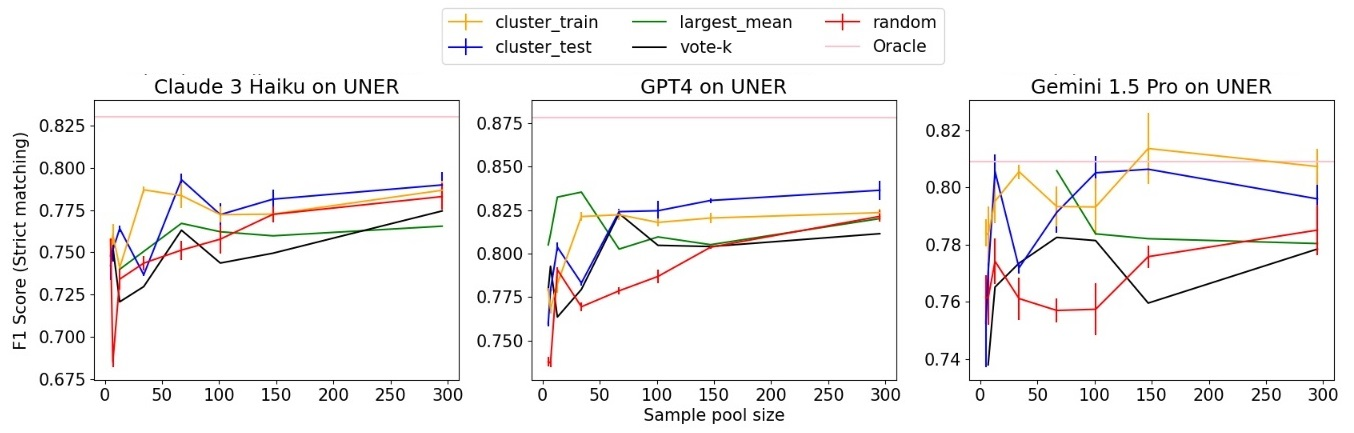}
    \caption{Results for NER using Claude 3 Haiku (left), GPT4 (middle) and Gemini 1.5 Pro (right) on UNER, as a function of the size of sample pool. In methods with a random component we run 3 trials and plot error bars showing the standard deviation. Oracle: using the full training set as the pool.}
    \label{fig:uner_results}
\end{figure*}

Figure~\ref{fig:uner_results} displays the results, reinforcing our conclusions from the main text.
